# Supplementary material for: Do accretion-powered stellar winds help spin down T Tauri stars?
Source: arXiv:2504.03374 source file (2025-04-04)
Supplement: Supplementary file 1 [file appendix.tex]

% \section{Stellar mass dependence of the equilibrium state}

% We have tested the dependence of the equilibrium state on the stellar mass.
% The mass dependence of the equilibrium state for the no-wind and wind scenario is relatively small compared to the dependence on the value of $W$ (see \fig{fig:theo}).
% For a stellar age of 2~Myr, the stellar mass ranges from $0.2~\mathrm{M_\odot}$ (blue lines) to $1.0~\mathrm{M_\odot}$ (red lines).



% \begin{figure}
%     \centering
%          \resizebox{\hsize}{!}{\includegraphics{assets/theo.pdf}}
%     \caption{
%     Equilibrium state values of $R_\mathrm{t}/R_\mathrm{co}$ over a range of stellar accretion rates.
%     We compare different stellar masses, $0.2~\mathrm{M_\odot}$ and $1.0~\mathrm{M_\odot}$. The magnetic field strength is 0.5~kG.
%     }
%     \label{fig:theo}
% \end{figure}




% \section{Comparison with hydrodynamic models}

% % To test the theoretical model, we compare the predictions made in \sref{sec:spin_model} with the hydrodynamic TAPIR code \citep[][]{ragossnig20, Steiner21, Gehrig2022}.
% % The TAPIR code combines stellar and disk evolution models self-consistently and can accurately calculate the values of $\Mdot$ and $R_\mathrm{t}$.
% % Thus, it is well-suited to verify the predictions made in this study.
% % In \fig{fig:demo}, we show the torque (in units of the stellar angular momentum) evolution of the no-wind (blue lines) and wind (red lines) scenarios close to the equilibrium state (solid lines) and when including parameter variations.
% % In its equilibrium state, the $0.7~\mathrm{M_\odot}$ star has an accretion rate of $\Mdot = 3.0 \times 10^{-9}~\Msolpyr$ and a magnetic field strength of 0.5~kG.
% % The dashed line ("$\mathrm{mod_{up}}$"), showing a spin-up torque, corresponds to an increase of $\Mdot$ by a factor of 2 and a decrease of $B_\star$ by a factor of 3 compared to the equilibrium values.
% % The dash-dotted line ("$\mathrm{mod_{down}}$"), showing a spin-down torque, corresponds to a decrease of $\Mdot$ by a factor of 2 and an increase of $B_\star$ by a factor of 3 compared to the equilibrium values.


% To test the theoretical model, we compare the predictions made in \sref{sec:spin_model} with the hydrodynamic TAPIR code \citep[][]{ragossnig20, Steiner21, Gehrig2022}.
% The TAPIR code combines stellar and disk evolution models self-consistently and can accurately calculate the values of $\Mdot$ and $R_\mathrm{t}$.
% Thus, it is well-suited to verify the predictions made in this study.
% In \fig{fig:demo}, we show the torque (in units of the stellar angular momentum) evolution of the no-wind (blue lines) and wind (red lines) scenarios close to the equilibrium state.
% The $0.7~\mathrm{M_\odot}$ star has an initial accretion rate of $\Mdot = 3.0 \times 10^{-9}~\Msolpyr$, a magnetic field strength of 0.5~kG, and an age of $\tau_\mathrm{age} = 2$~Myr.
% During its evolution the stellar radius and accretion rate decrease changing the equilibrium target.
% The resulting torque, however, is small.
% For comparison, the shaded area shows the expected torque range when including unpredictable parameter variations (see \sref{sec:uncert}).


% \begin{figure}
%     \centering
%          \resizebox{\hsize}{!}{\includegraphics{assets/demo2.pdf}}
%     \caption{
%     Torque (in units of the stellar angular momentum) evolution of the no-wind (blue lines) and wind (red lines) scenarios close to the equilibrium state.
%     The stellar mass is $0.7~\mathrm{M_\odot}$ and the magnetic field strength is $0.5$~kG.
%     For comparison, the shaded area shows the predicted torque range for the short-term variations of the model parameters. 
%     }
%     \label{fig:demo}
% \end{figure}





% \section{Literature uncertainty of observational parameters}

% In \tab{tab:errors}, we summarize the intrinsic variations and uncertainties, $\delta_\mathrm{var}$, of the observational parameters required to build the spin population model. 

% \begin{table}[ht]
% \centering
% \caption{Variations and uncertainties, $\delta_\mathrm{var}$, of the observational parameters. In the SPM, the respective quantity $X$ may vary between $X/\delta_\mathrm{var}$ and $X\times\delta_\mathrm{var}$ ($X-\delta_\mathrm{var}$ and $X+\delta_\mathrm{var}$, in case of $R_\mathrm{t}$).}        
% \begin{tabular}{c | c | c}
% \hline\hline
% Parameter & $\delta_\mathrm{var}$ & Ref \\
% \hline

% $\Mdot$ & 0.35~dex & \cite{Manara22} \\
% $B_\star$ & 0.48~dex & \cite{Johnstone14} \\
% $M_\star$ & 0.10~dex & \cite{Alcala2017} \\
% $R_\star$ & 0.09~dex & \cite{Alcala2017} \\
% $\Omega_\star$ & 0.01~dex & \cite{Bowler2023} \\
% $R_\mathrm{t}$ & $0.2\times R_\star$ & see \sref{sec:obs} \\
% \hline\hline                                            
% \end{tabular}
% \label{tab:errors}  
% \end{table}
